# Supplementary material for: DreamPBR: Text-driven Generation of High-resolution SVBRDF with Multi-modal Guidance
Source: arXiv:2404.14676 source file (2024-07-01)
Supplement: Supplementary file 1 [file 7_supplement.tex]

% !TeX root = ../main.tex

\clearpage

\pagebreak

\twocolumn[
\begin{center}
  \huge \textbf{Supplementary Materials for DreamPBR: \\Text-driven Generation of High-resolution SVBRDF with Multi-modal Guidance} 
\end{center}
\vskip 2em
]

\paragraph{Supplementary results for random generation.} We provide rando\-mly generated samples for each category in \autoref{fig:random_supple}. These samples were produced using the prompt ``a PBR material of [category]," covering the ten predefined categories we established.

\paragraph{Supplementary results for text-only generation.} We exhibit the results of text-only generation for various materials in \autoref{fig:txt_supple}. The first column lists the prompts used for each material.

\paragraph{Supplementary results of pixel control.} We display the pixel control results within the tile category in \autoref{fig:pixel_supple}. Each row begins with a binary image, and the uniform prompt used was ``a PBR material of tile."

\paragraph{Supplementary results of style control.} Additional style control outcomes are shown in \autoref{fig:style_supple}. The styled images appear in the first column, with corresponding material descriptions provided beneath each image.

\paragraph{Supplementary results of shape control.} We showcase additional shape control outcomes in \autoref{fig:shape_supple}. Each multimodal control signal, including the binary and RGB images, is positioned next to the SVBRDF texture, demonstrating control beyond textual descriptions.
\newpage

\newcommand{\SupWidthRan}{3.4cm} 
\newcommand{\SupWidthTxt}{3.2cm} 

% Random Gerenation
\begin{figure*}[tb]
  \centering
  \bgroup
   
  \setlength\tabcolsep{0.5pt} 
  \begin{tabular}{
      m{0.3cm}
      m{\SupWidthRan}
      m{\SupWidthRan}
      m{\SupWidthRan}
      m{\SupWidthRan}
      m{\SupWidthRan}
      }
  \raisebox{+0.8\height}{\rotatebox[origin=c]{90}{\small{Brick}}} &
  \includegraphics[width=\SupWidthRan]{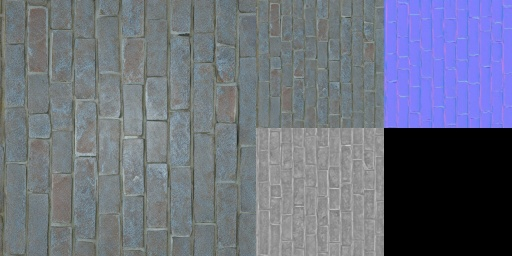} &
  \includegraphics[width=\SupWidthRan]{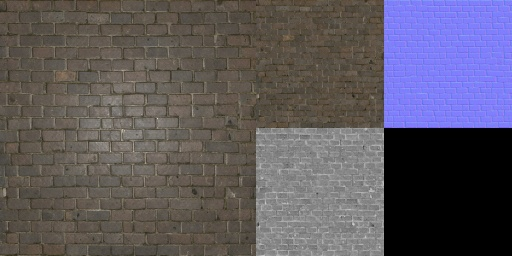} &
  \includegraphics[width=\SupWidthRan]{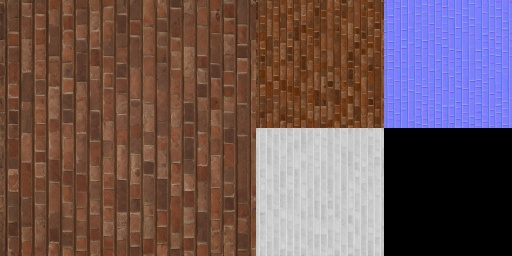} &  
  \includegraphics[width=\SupWidthRan]{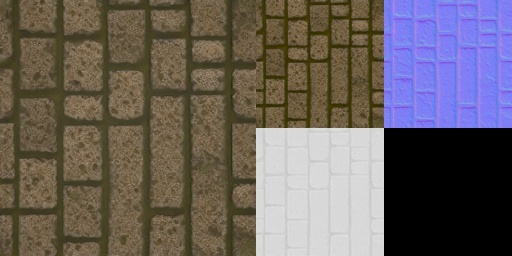} &
  \includegraphics[width=\SupWidthRan]{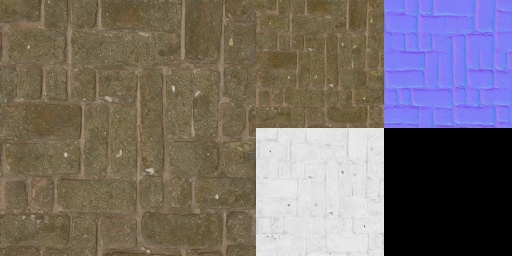} \\

  \raisebox{+0.8\height}{\rotatebox[origin=c]{90}{\small{Fabric}}} &
  \includegraphics[width=\SupWidthRan]{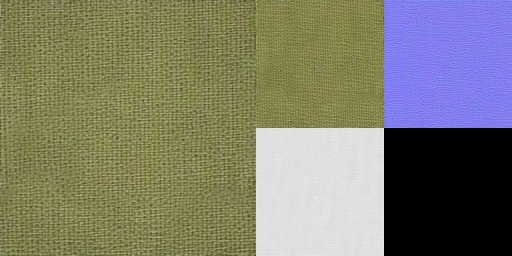} &
  \includegraphics[width=\SupWidthRan]{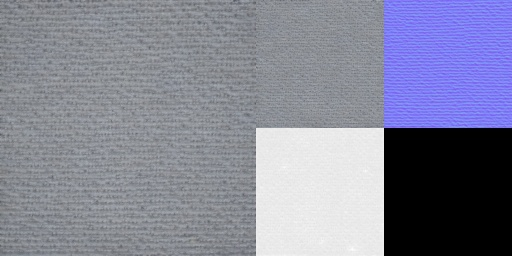} &
  \includegraphics[width=\SupWidthRan]{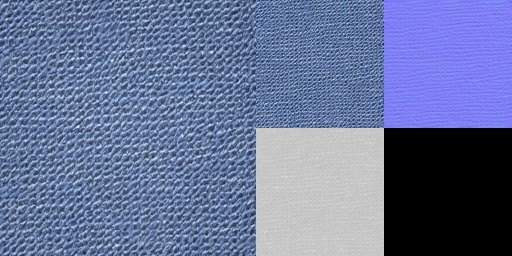} &
  \includegraphics[width=\SupWidthRan]{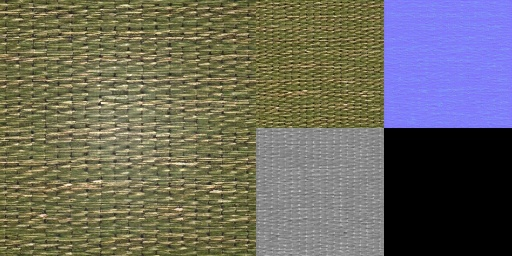} &
  \includegraphics[width=\SupWidthRan]{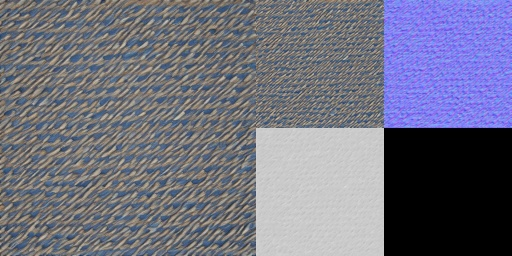} \\

  \raisebox{+0.8\height}{\rotatebox[origin=c]{90}{\small{Ground}}} &
  \includegraphics[width=\SupWidthRan]{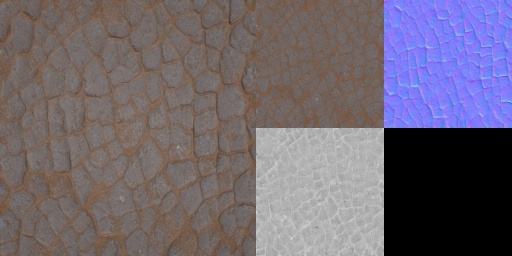} &
  \includegraphics[width=\SupWidthRan]{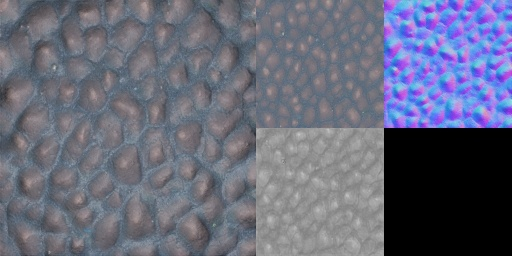} &
  \includegraphics[width=\SupWidthRan]{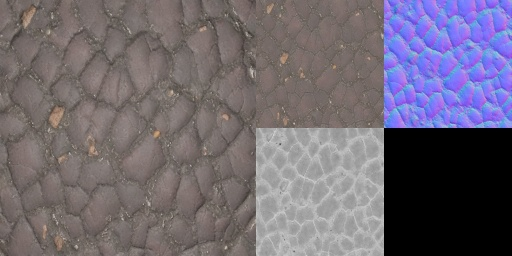} &
  \includegraphics[width=\SupWidthRan]{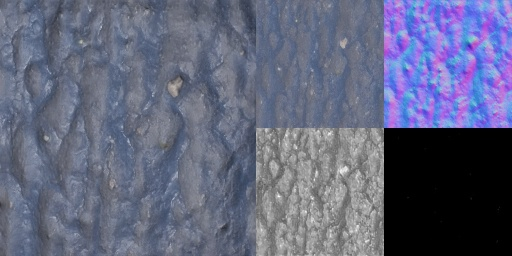} &
  \includegraphics[width=\SupWidthRan]{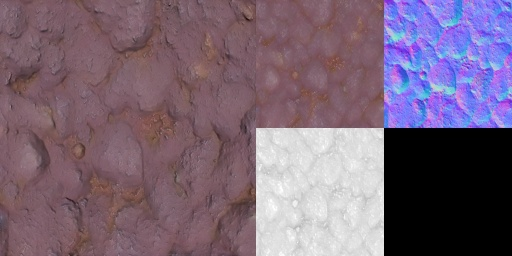} \\

  \raisebox{+0.8\height}{\rotatebox[origin=c]{90}{\small{Leather}}} &
  \includegraphics[width=\SupWidthRan]{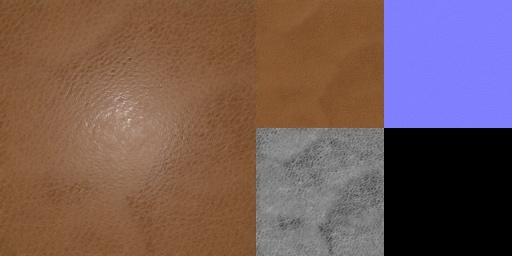} &
  \includegraphics[width=\SupWidthRan]{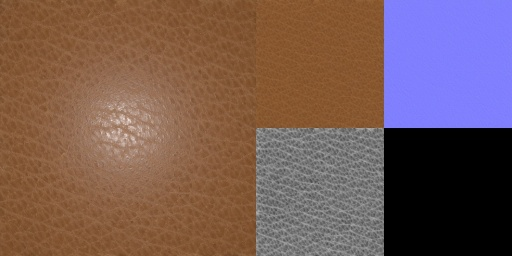} &
  \includegraphics[width=\SupWidthRan]{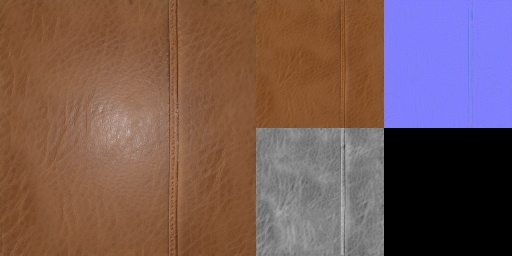} &
  \includegraphics[width=\SupWidthRan]{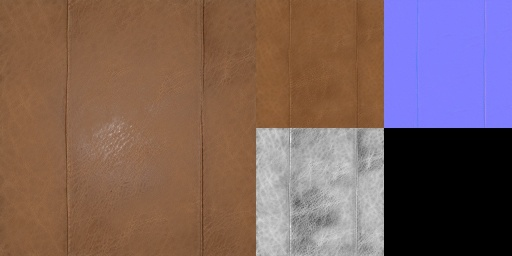} &
  \includegraphics[width=\SupWidthRan]{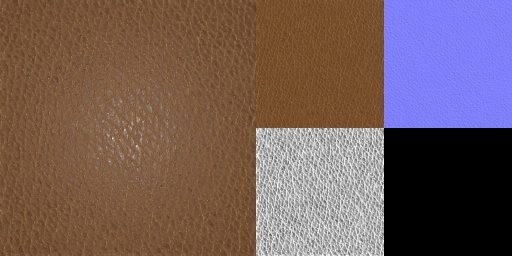} \\

  \raisebox{+0.8\height}{\rotatebox[origin=c]{90}{\small{Metal}}} &
  \includegraphics[width=\SupWidthRan]{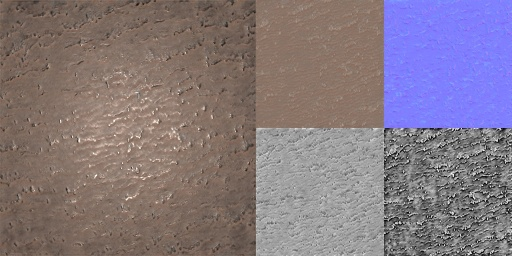} &
  \includegraphics[width=\SupWidthRan]{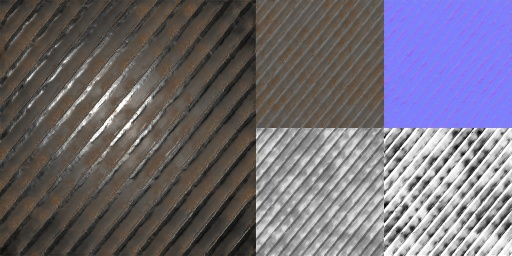} &
  \includegraphics[width=\SupWidthRan]{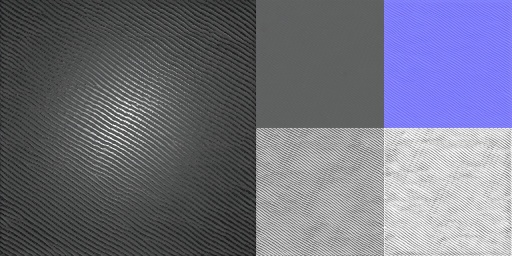} &
  \includegraphics[width=\SupWidthRan]{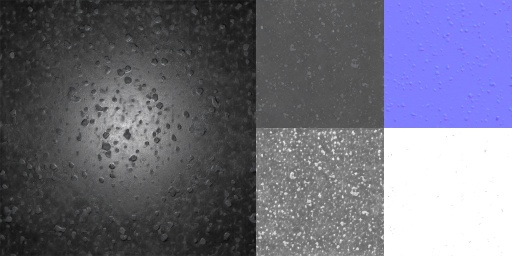} &
  \includegraphics[width=\SupWidthRan]{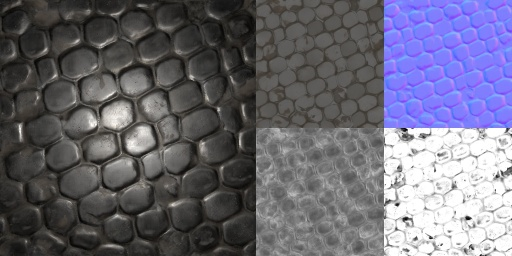} \\

  \raisebox{+0.8\height}{\rotatebox[origin=c]{90}{\small{Organic}}} &
  \includegraphics[width=\SupWidthRan]{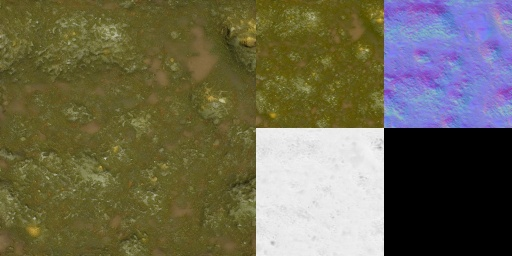} &
  \includegraphics[width=\SupWidthRan]{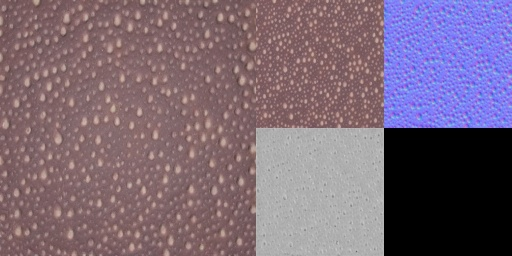} &
  \includegraphics[width=\SupWidthRan]{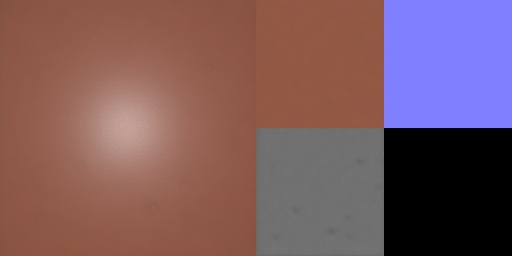} &
  \includegraphics[width=\SupWidthRan]{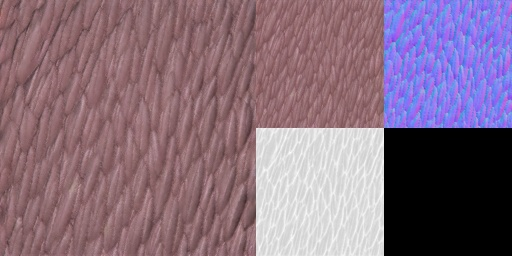} &
  \includegraphics[width=\SupWidthRan]{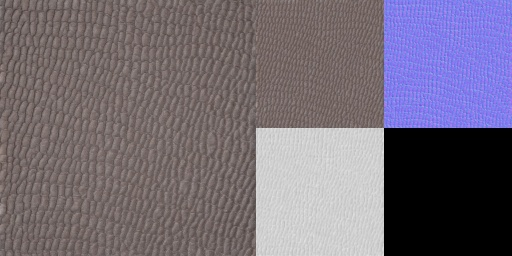} \\

  \raisebox{+0.8\height}{\rotatebox[origin=c]{90}{\small{Plastic}}} &
  \includegraphics[width=\SupWidthRan]{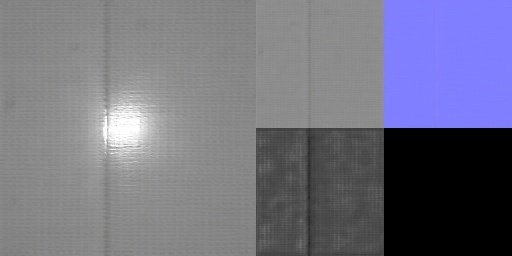} &
  \includegraphics[width=\SupWidthRan]{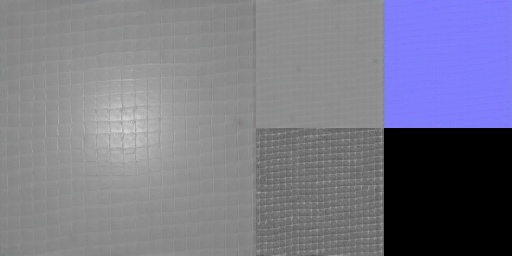} &
  \includegraphics[width=\SupWidthRan]{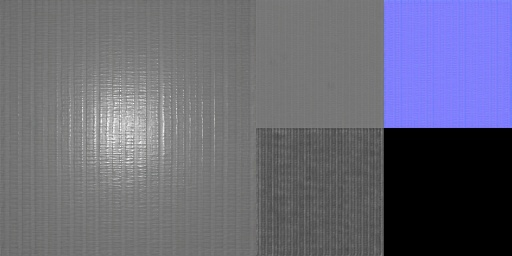} &
  \includegraphics[width=\SupWidthRan]{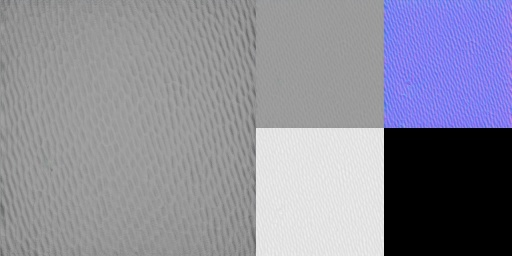} &
  \includegraphics[width=\SupWidthRan]{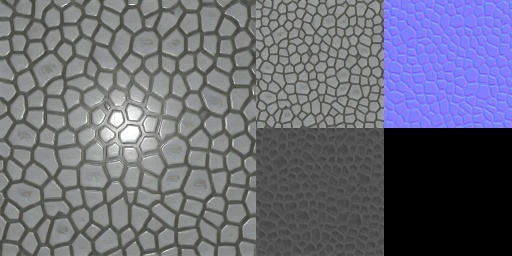} \\

  \raisebox{+0.8\height}{\rotatebox[origin=c]{90}{\small{Tile}}} &
  \includegraphics[width=\SupWidthRan]{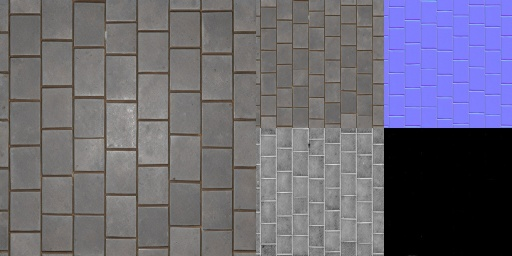} &
  \includegraphics[width=\SupWidthRan]{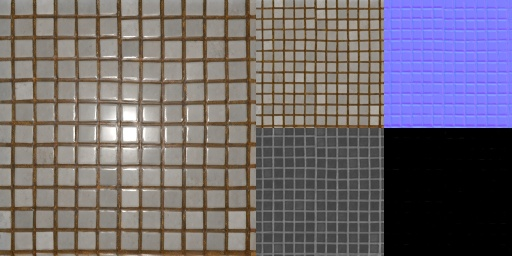} &
  \includegraphics[width=\SupWidthRan]{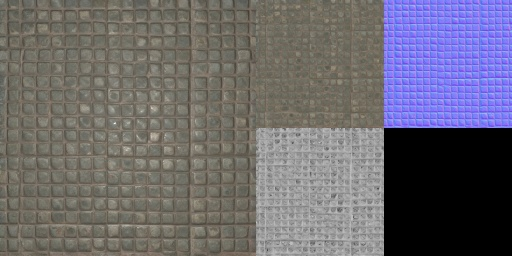} &
  \includegraphics[width=\SupWidthRan]{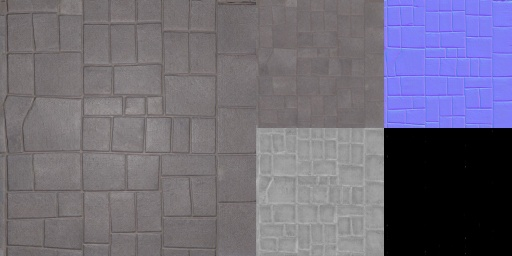} &
  \includegraphics[width=\SupWidthRan]{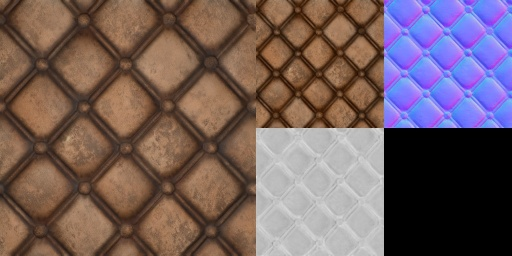} \\

  \raisebox{+0.8\height}{\rotatebox[origin=c]{90}{\small{Wall}}} &
  \includegraphics[width=\SupWidthRan]{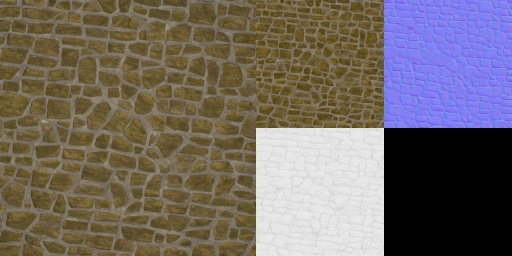} &
  \includegraphics[width=\SupWidthRan]{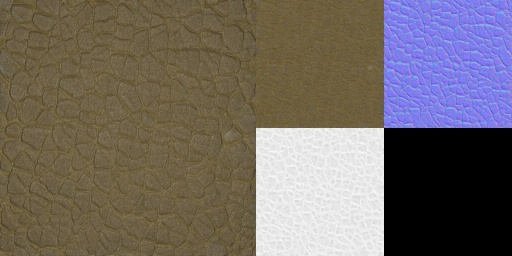} &
  \includegraphics[width=\SupWidthRan]{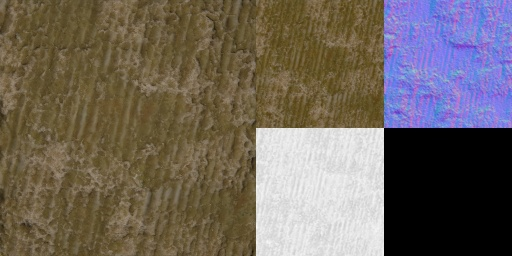} &
  \includegraphics[width=\SupWidthRan]{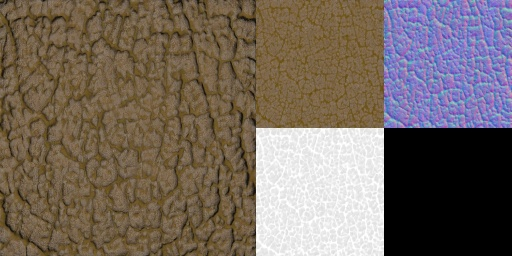} &
  \includegraphics[width=\SupWidthRan]{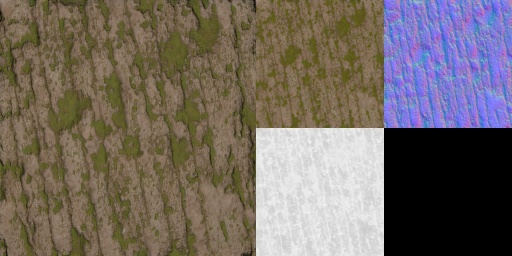} \\

  \raisebox{+0.8\height}{\rotatebox[origin=c]{90}{\small{Wood}}} &
  \includegraphics[width=\SupWidthRan]{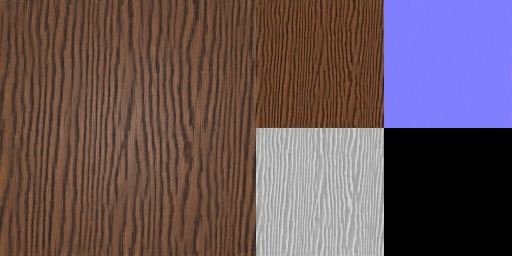} &
  \includegraphics[width=\SupWidthRan]{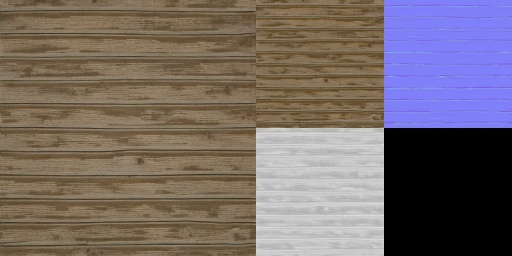} &
  \includegraphics[width=\SupWidthRan]{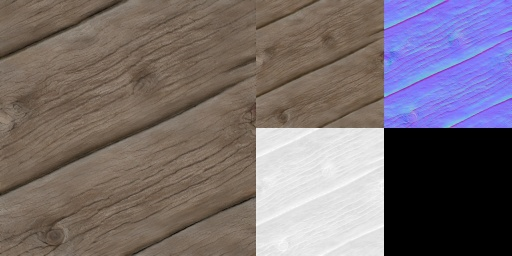} &
  \includegraphics[width=\SupWidthRan]{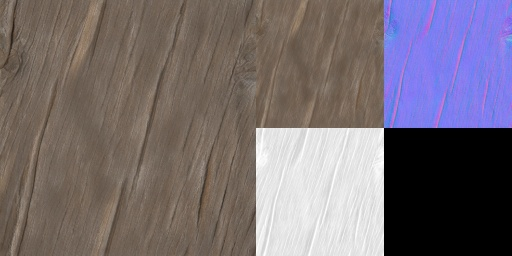} &
  \includegraphics[width=\SupWidthRan]{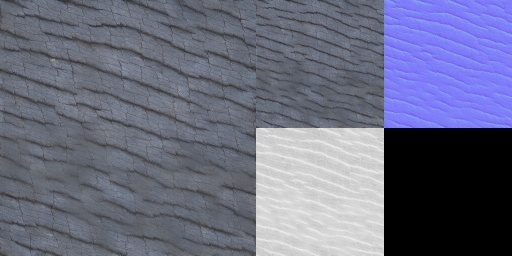} \\
  
  \end{tabular}
  \egroup
\caption{Additional results for random generation.}
\Description{}
\label{fig:random_supple}
\end{figure*}

% txt control
\begin{figure*}[tb]
  \centering
  \bgroup
   
  \setlength\tabcolsep{0.5pt} 
  \begin{tabular}{
      >{\raggedright\arraybackslash}m{1.5cm} 
      m{\SupWidthTxt}
      m{\SupWidthTxt}
      m{\SupWidthTxt}
      m{\SupWidthTxt}
      m{\SupWidthTxt}
      }
  \scriptsize\textit{a PBR material of brick, blue painted bricks, vivid, outdoor, wall} & 
  \includegraphics[width=\SupWidthTxt]{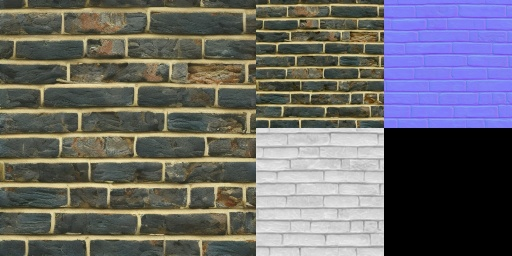} &
  \includegraphics[width=\SupWidthTxt]{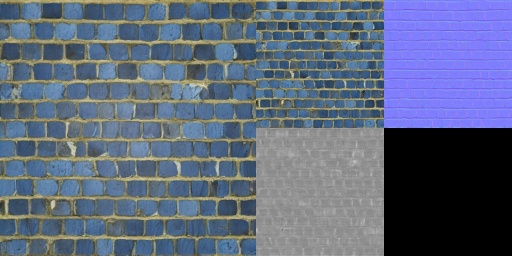} &
  \includegraphics[width=\SupWidthTxt]{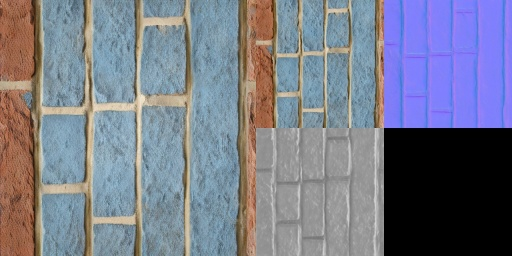} &
  \includegraphics[width=\SupWidthTxt]{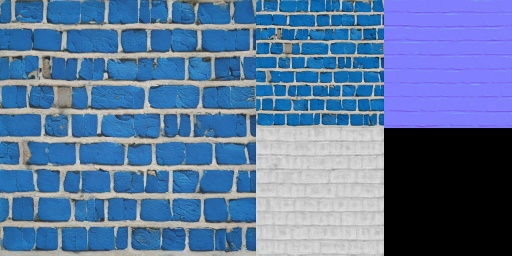} &
  \includegraphics[width=\SupWidthTxt]{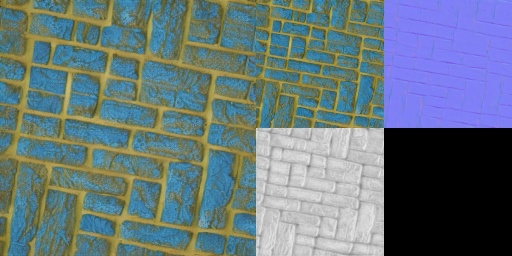} \\

  \scriptsize\textit{a PBR material of brick, designed brick, floor, outdoor, detailed carving, paving} & 
  \includegraphics[width=\SupWidthTxt]{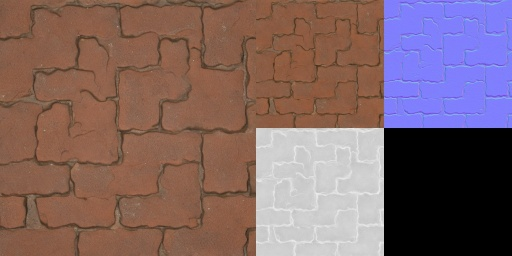} &
  \includegraphics[width=\SupWidthTxt]{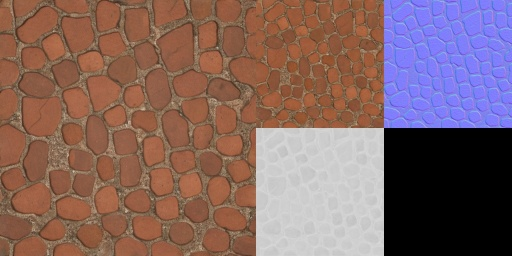} &
  \includegraphics[width=\SupWidthTxt]{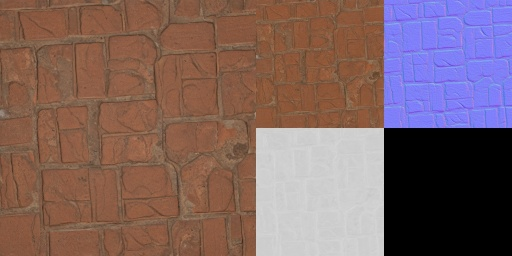} &
  \includegraphics[width=\SupWidthTxt]{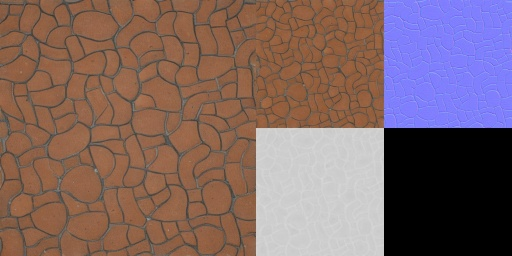} &
  \includegraphics[width=\SupWidthTxt]{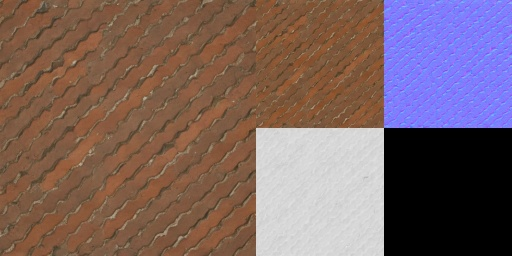} \\

  \scriptsize\textit{a PBR material of fabric, embroidered linen, delicate, indoor, tablecloth} & 
  \includegraphics[width=\SupWidthTxt]{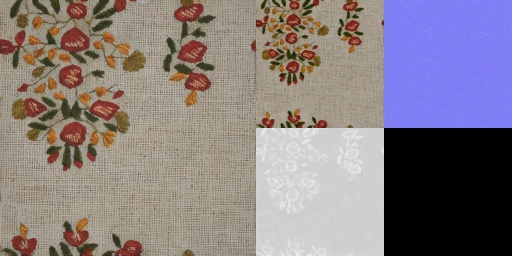} &
  \includegraphics[width=\SupWidthTxt]{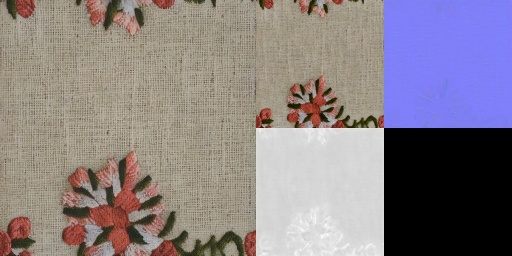} &
  \includegraphics[width=\SupWidthTxt]{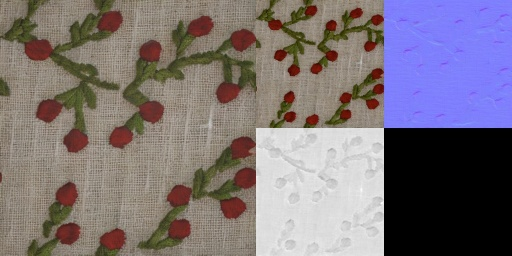} &
  \includegraphics[width=\SupWidthTxt]{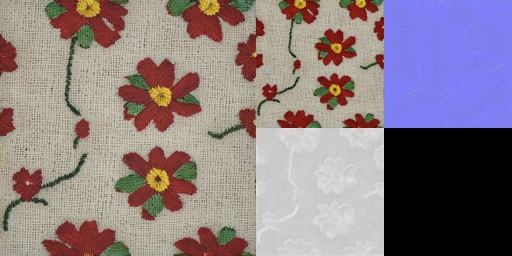} &
  \includegraphics[width=\SupWidthTxt]{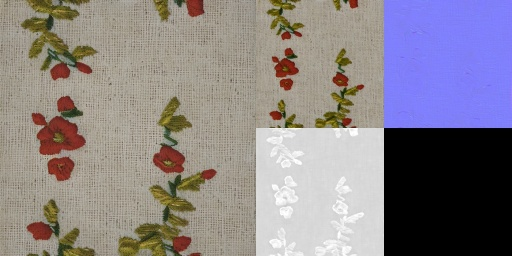} \\

  \scriptsize\textit{a PBR material of fabric, flannel shirt texture, cozy, clothing} & 
  \includegraphics[width=\SupWidthTxt]{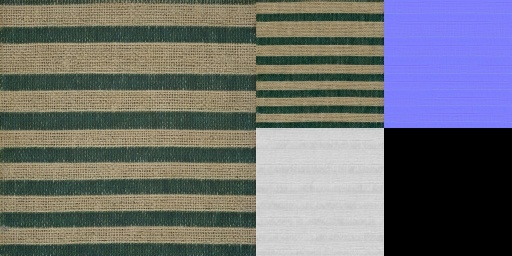} &
  \includegraphics[width=\SupWidthTxt]{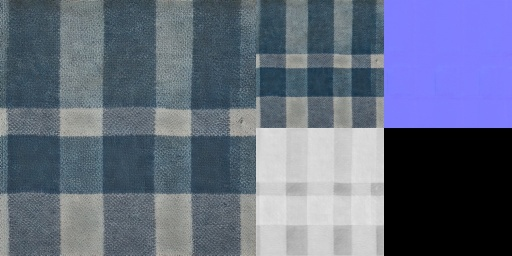} &
  \includegraphics[width=\SupWidthTxt]{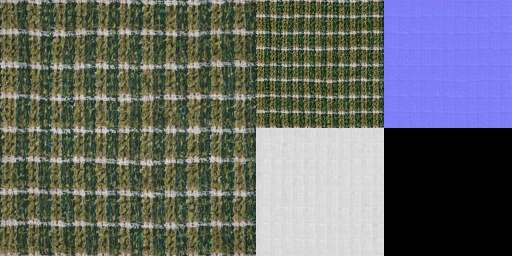} &
  \includegraphics[width=\SupWidthTxt]{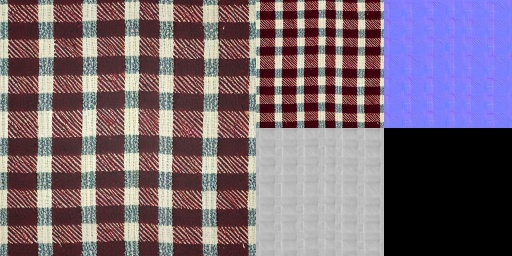} &
  \includegraphics[width=\SupWidthTxt]{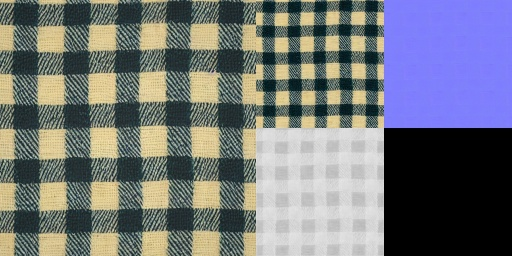} \\

  \scriptsize\textit{a PBR material of fabric, floral, dress, summery, clothing} & 
  \includegraphics[width=\SupWidthTxt]{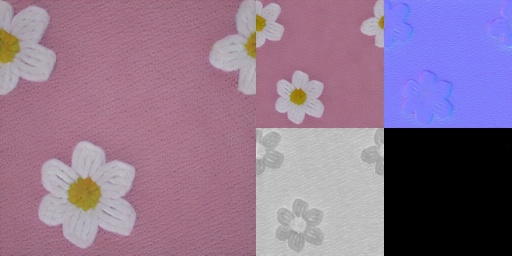} &
  \includegraphics[width=\SupWidthTxt]{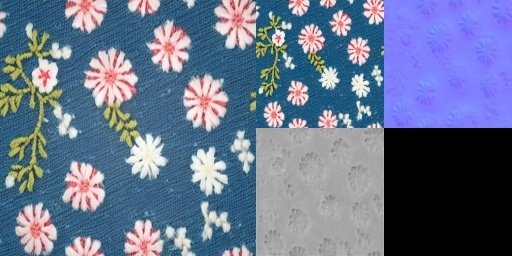} &
  \includegraphics[width=\SupWidthTxt]{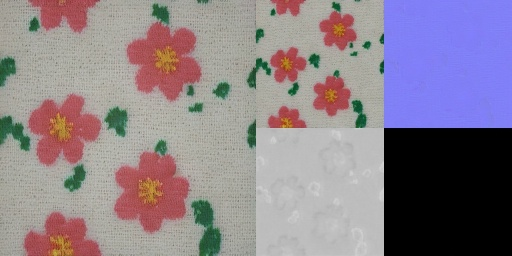} &
  \includegraphics[width=\SupWidthTxt]{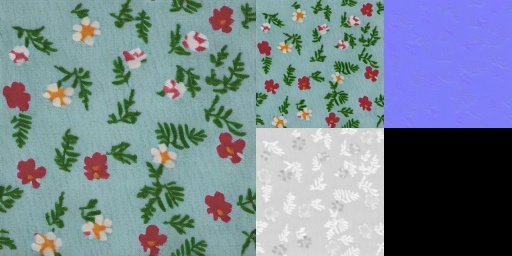} &
  \includegraphics[width=\SupWidthTxt]{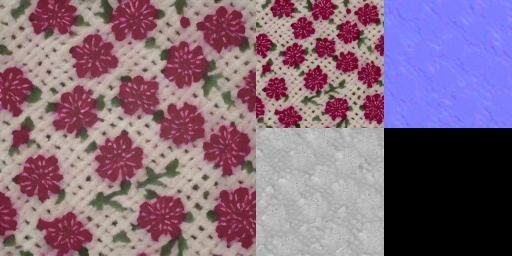} \\

  \scriptsize\textit{a PBR material of ground, marble floor tiles, polished, indoor, luxury} & 
  \includegraphics[width=\SupWidthTxt]{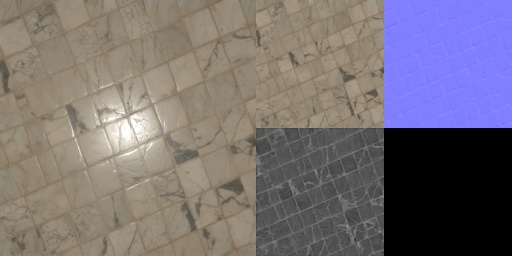} &
  \includegraphics[width=\SupWidthTxt]{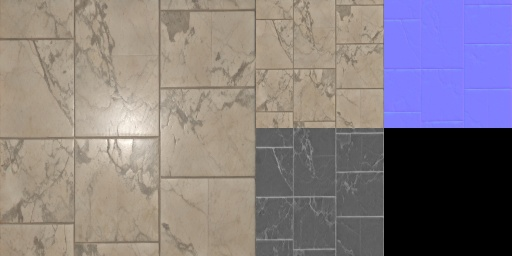} &
  \includegraphics[width=\SupWidthTxt]{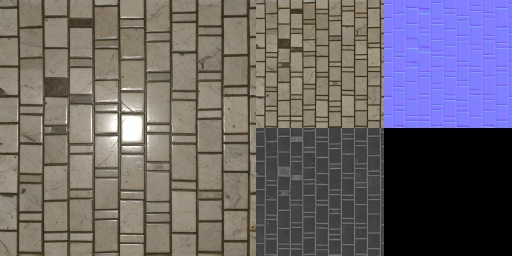} &
  \includegraphics[width=\SupWidthTxt]{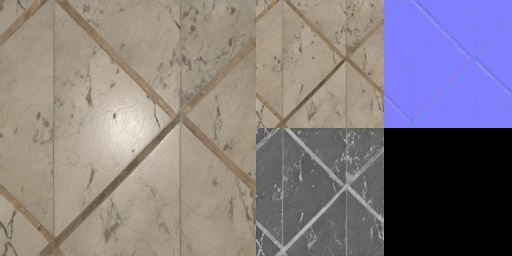} &
  \includegraphics[width=\SupWidthTxt]{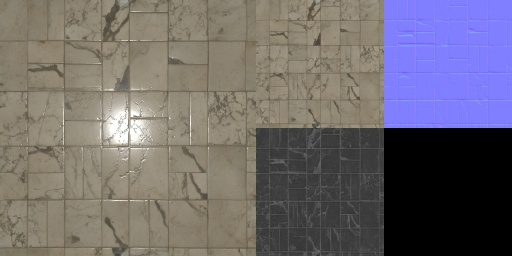} \\

  \scriptsize\textit{a PBR material of leather, animal, fashion, accessories} & 
  \includegraphics[width=\SupWidthTxt]{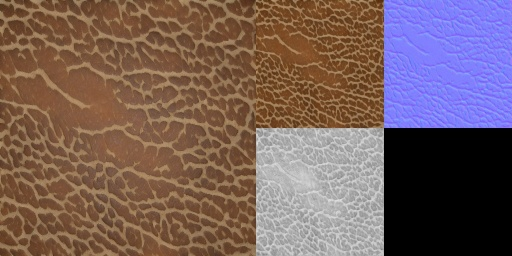} &
  \includegraphics[width=\SupWidthTxt]{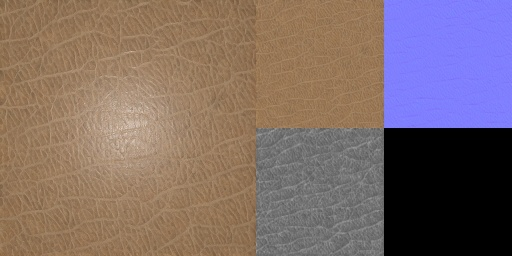} &
  \includegraphics[width=\SupWidthTxt]{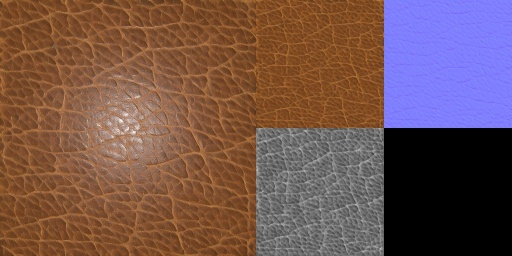} &
  \includegraphics[width=\SupWidthTxt]{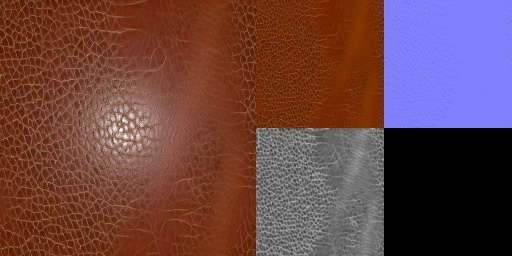} &
  \includegraphics[width=\SupWidthTxt]{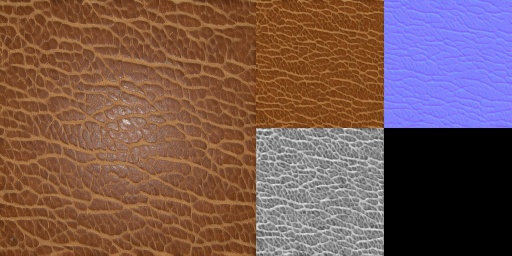} \\
  
  \scriptsize\textit{a PBR material of metal, fancy diamond metal} & 
  \includegraphics[width=\SupWidthTxt]{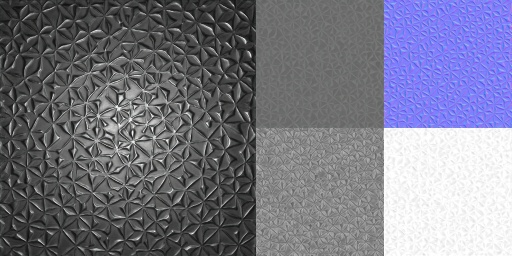} &
  \includegraphics[width=\SupWidthTxt]{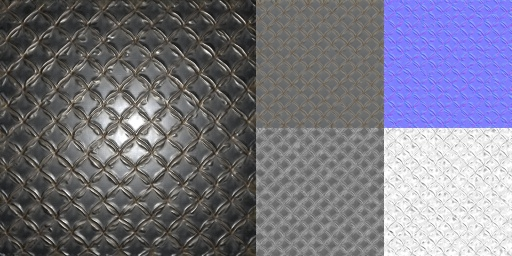} &
  \includegraphics[width=\SupWidthTxt]{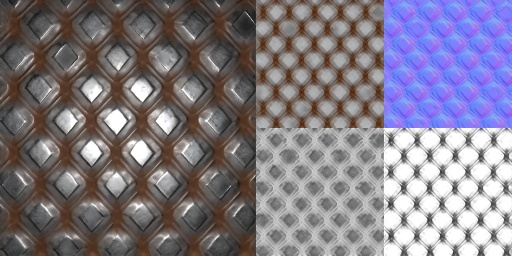} &
  \includegraphics[width=\SupWidthTxt]{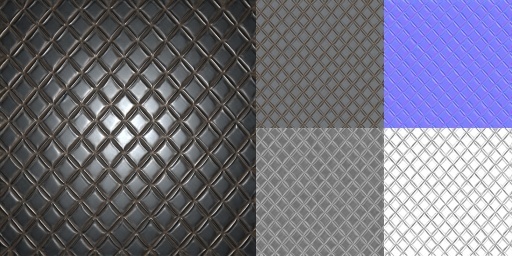} &
  \includegraphics[width=\SupWidthTxt]{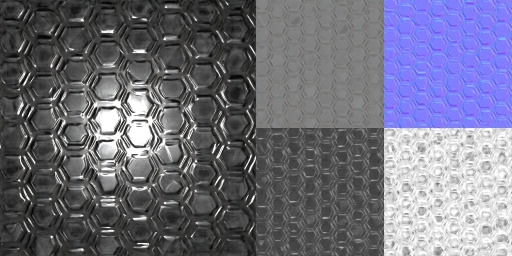} \\

  \scriptsize\textit{a PBR material of tile, art deco style tiles, vintage, indoor, decorative} & 
  \includegraphics[width=\SupWidthTxt]{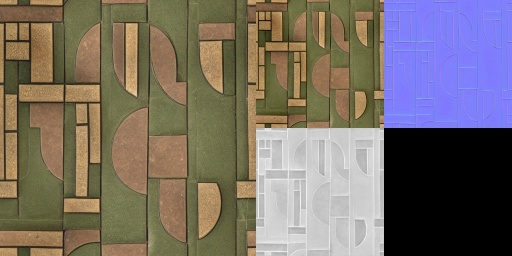} &
  \includegraphics[width=\SupWidthTxt]{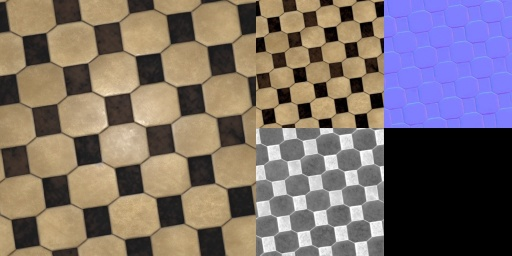} &
  \includegraphics[width=\SupWidthTxt]{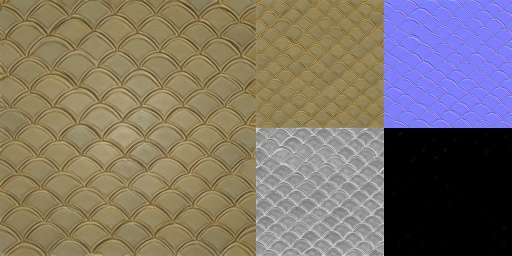} &
  \includegraphics[width=\SupWidthTxt]{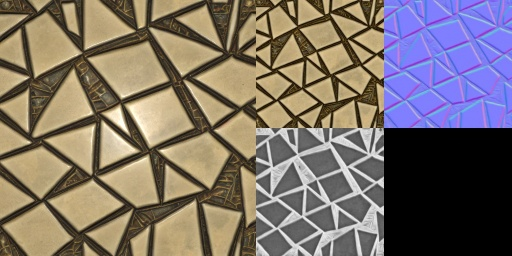} &
  \includegraphics[width=\SupWidthTxt]{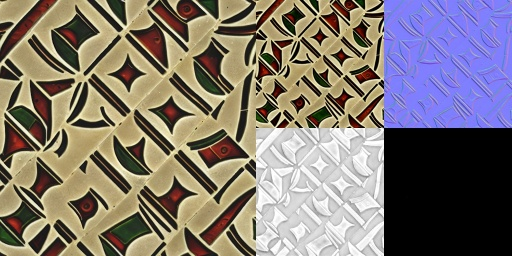} \\

  \scriptsize\textit{a PBR material of tile, patterned bw vinyl, floors} & 
  \includegraphics[width=\SupWidthTxt]{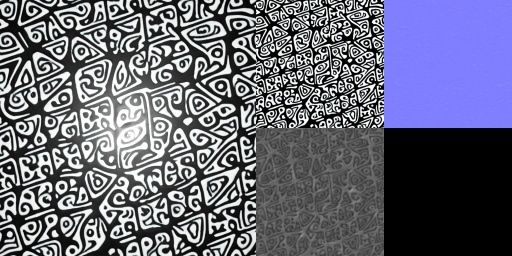} &
  \includegraphics[width=\SupWidthTxt]{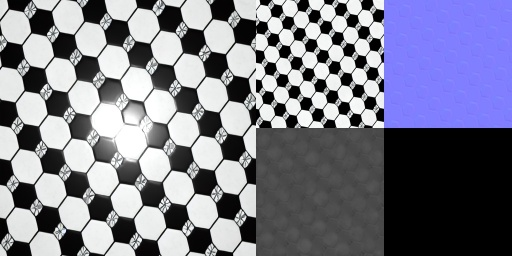} &
  \includegraphics[width=\SupWidthTxt]{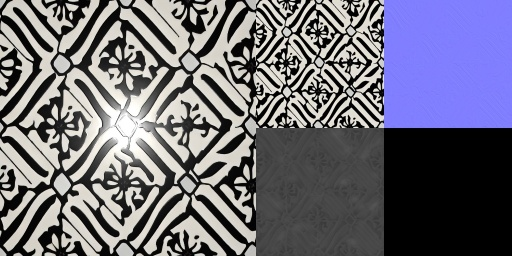} &
  \includegraphics[width=\SupWidthTxt]{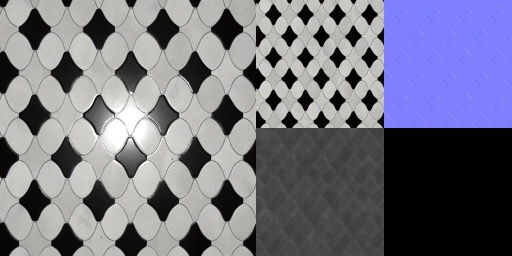} &
  \includegraphics[width=\SupWidthTxt]{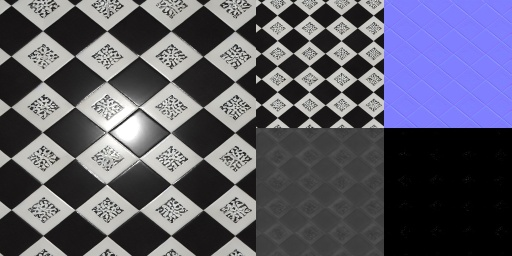} \\

  \scriptsize\textit{a PBR material of wall, wallpaper, royalty, noble, patterned, indoor, historic} & 
  \includegraphics[width=\SupWidthTxt]{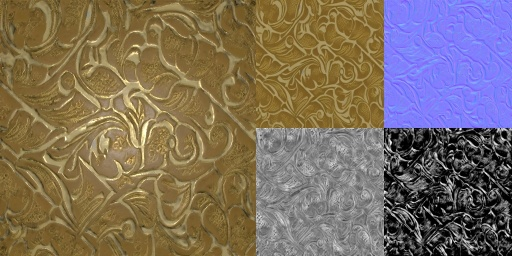} &
  \includegraphics[width=\SupWidthTxt]{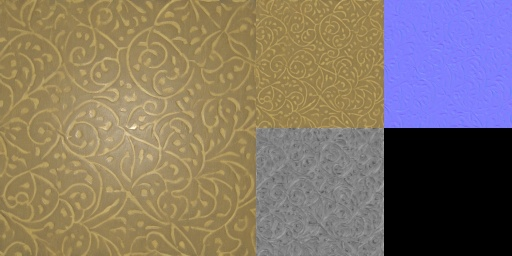} &
  \includegraphics[width=\SupWidthTxt]{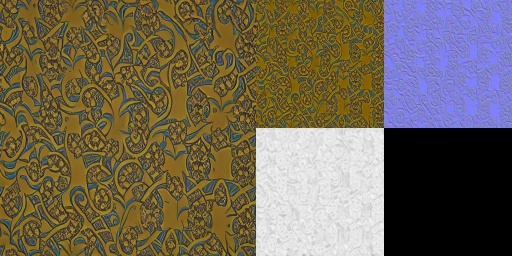} &
  \includegraphics[width=\SupWidthTxt]{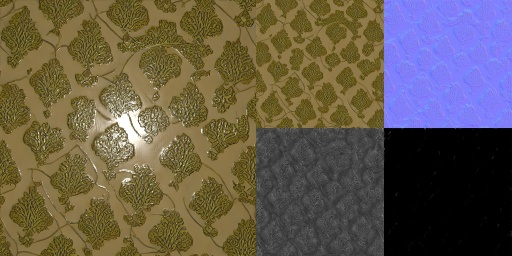} &
  \includegraphics[width=\SupWidthTxt]{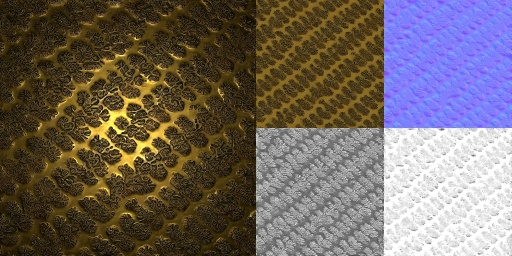} \\

\end{tabular}
\egroup
\caption{Additional results for text generation.}
\Description{}
\label{fig:txt_supple}
\end{figure*}

% pixel control
\begin{figure*}[tb]
  \centering
  \bgroup
   
  \setlength\tabcolsep{0.5pt} 
  \begin{tabular}{
      m{1.6cm} 
      m{\SupWidthTxt}
      m{\SupWidthTxt}
      m{\SupWidthTxt}
      m{\SupWidthTxt}
      m{\SupWidthTxt}
      }
  \includegraphics[width=1.6cm]{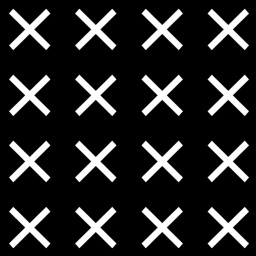} &
  \includegraphics[width=\SupWidthTxt]{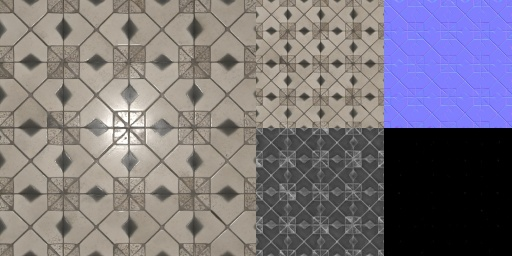} &
  \includegraphics[width=\SupWidthTxt]{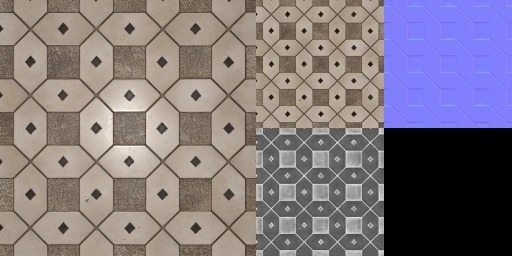} &
  \includegraphics[width=\SupWidthTxt]{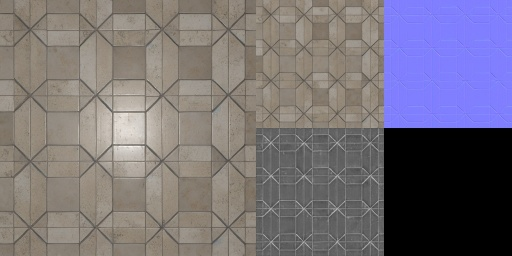} &
  \includegraphics[width=\SupWidthTxt]{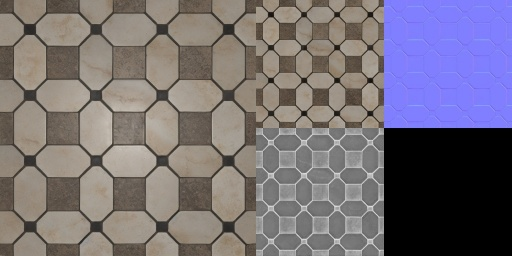} &
  \includegraphics[width=\SupWidthTxt]{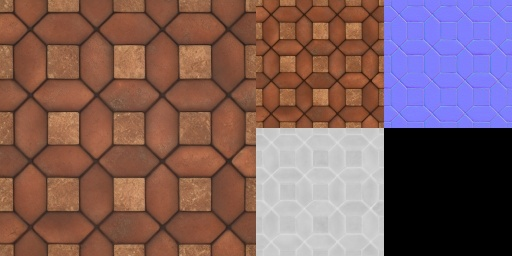} \\

  \includegraphics[width=1.6cm]{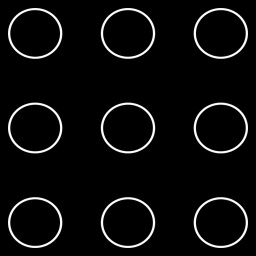} &
  \includegraphics[width=\SupWidthTxt]{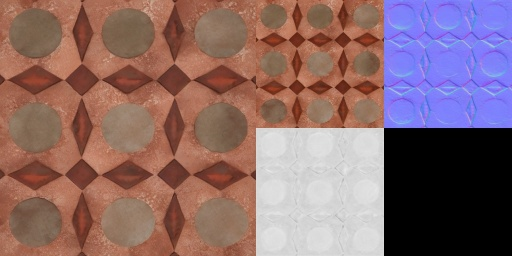} &
  \includegraphics[width=\SupWidthTxt]{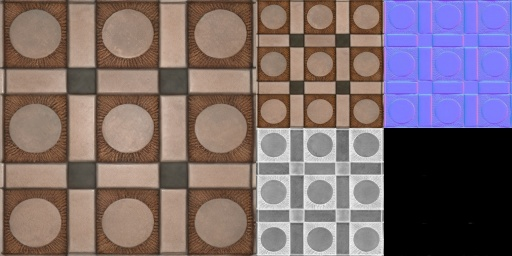} &
  \includegraphics[width=\SupWidthTxt]{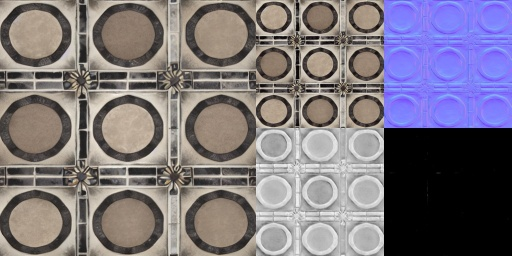} &
  \includegraphics[width=\SupWidthTxt]{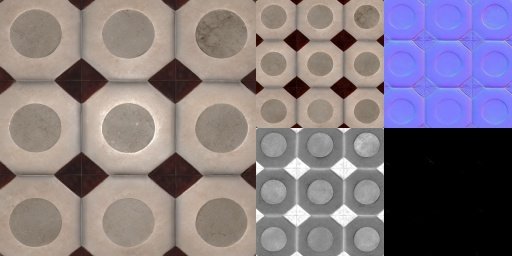} &
  \includegraphics[width=\SupWidthTxt]{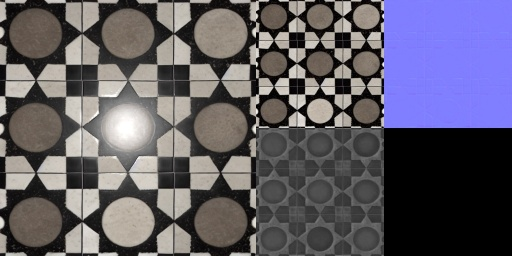} \\

  \includegraphics[width=1.6cm]{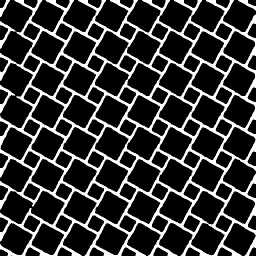} &
  \includegraphics[width=\SupWidthTxt]{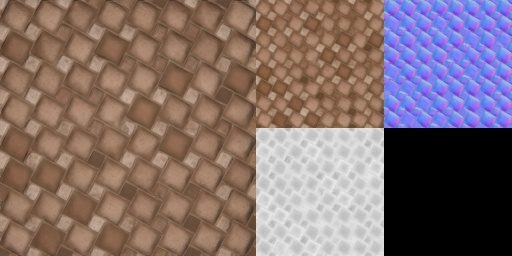} &
  \includegraphics[width=\SupWidthTxt]{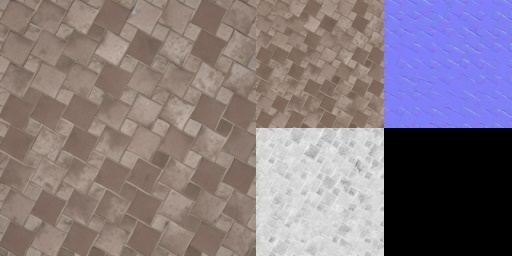} &
  \includegraphics[width=\SupWidthTxt]{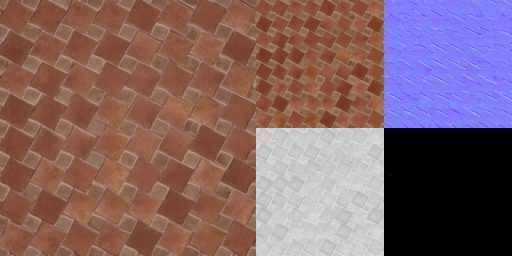} &
  \includegraphics[width=\SupWidthTxt]{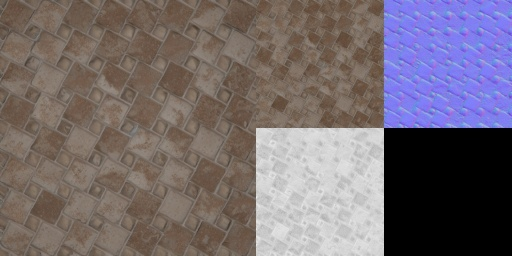} &
  \includegraphics[width=\SupWidthTxt]{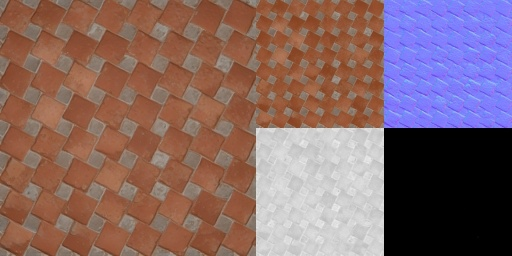} \\

  \includegraphics[width=1.6cm]{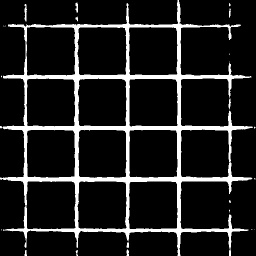} &
  \includegraphics[width=\SupWidthTxt]{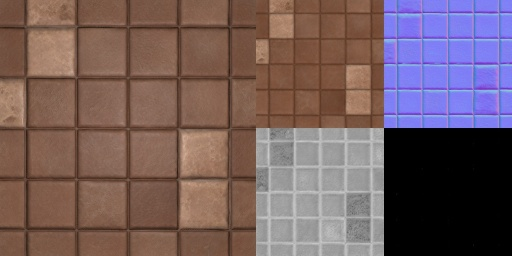} &
  \includegraphics[width=\SupWidthTxt]{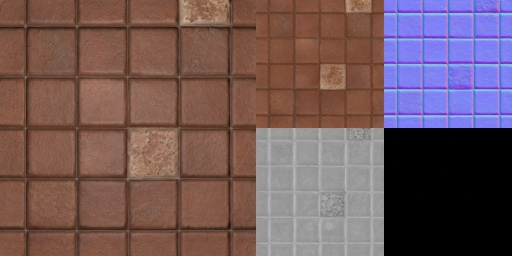} &
  \includegraphics[width=\SupWidthTxt]{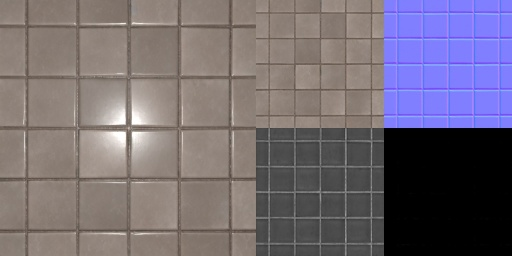} &
  \includegraphics[width=\SupWidthTxt]{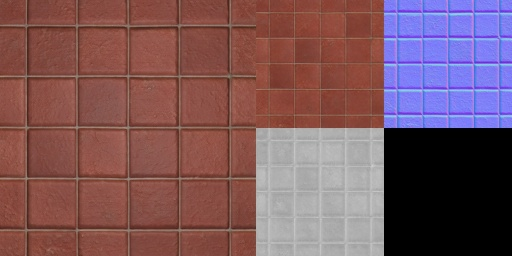} &
  \includegraphics[width=\SupWidthTxt]{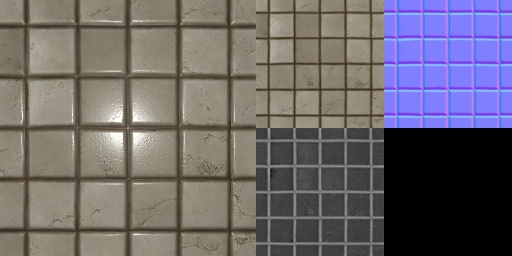} \\

\end{tabular}
\egroup
\caption{Additional results for pixel control.}
\Description{}
\label{fig:pixel_supple}
\end{figure*}

% style control
\begin{figure*}[tb]
  \centering
  \bgroup
   
  \setlength\tabcolsep{0.5pt} 
  \begin{tabular}{
      m{1.6cm} 
      m{\SupWidthTxt}
      m{\SupWidthTxt}
      m{\SupWidthTxt}
      m{\SupWidthTxt}
      m{\SupWidthTxt}
      }
  \includegraphics[width=1.6cm]{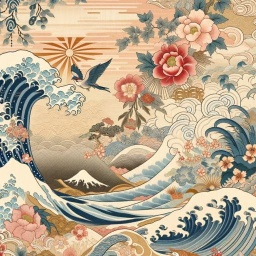} &
  \includegraphics[width=\SupWidthTxt]{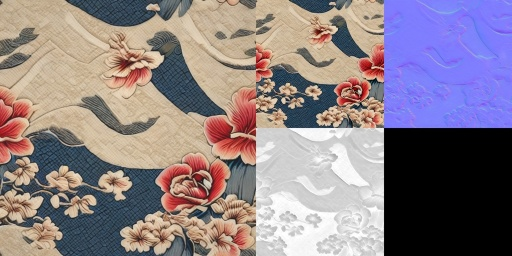} &
  \includegraphics[width=\SupWidthTxt]{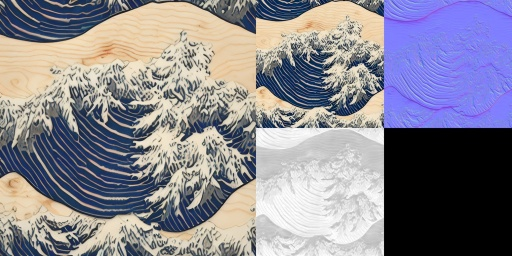} &
  \includegraphics[width=\SupWidthTxt]{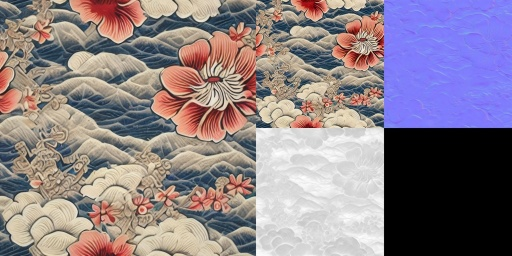} &
  \includegraphics[width=\SupWidthTxt]{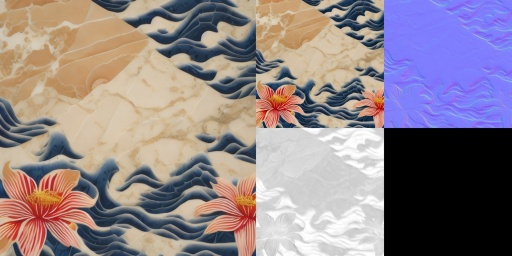} &
  \includegraphics[width=\SupWidthTxt]{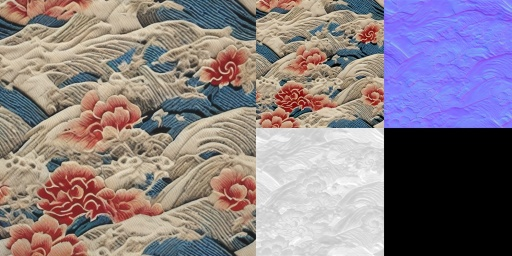} \\

  &
  \begin{minipage}{\SupWidthTxt}
    \centering
    \scriptsize\textit{a PBR material of leather} 
  \end{minipage} &
  \begin{minipage}{\SupWidthTxt}
    \centering
    \scriptsize\textit{a PBR material of wood, painted} 
  \end{minipage} &
  \begin{minipage}{\SupWidthTxt}
    \centering
    \scriptsize\textit{a PBR material of wall, wallpaper} 
  \end{minipage} &
  \begin{minipage}{\SupWidthTxt}
    \centering
    \scriptsize\textit{a PBR material of tile, marble} 
  \end{minipage} &
  \begin{minipage}{\SupWidthTxt}
    \centering
    \scriptsize\textit{a PBR material of fabric, carpet} 
  \end{minipage} \\
  \noalign{\smallskip}

  \includegraphics[width=1.6cm]{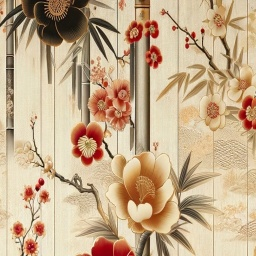} &
  \includegraphics[width=\SupWidthTxt]{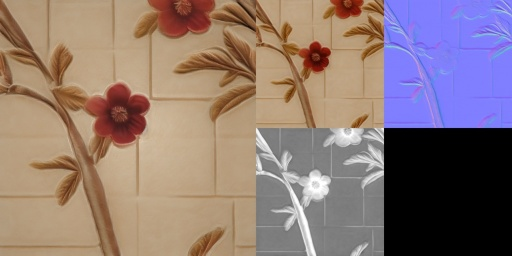} &
  \includegraphics[width=\SupWidthTxt]{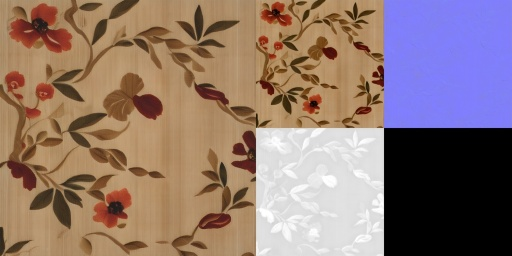} &
  \includegraphics[width=\SupWidthTxt]{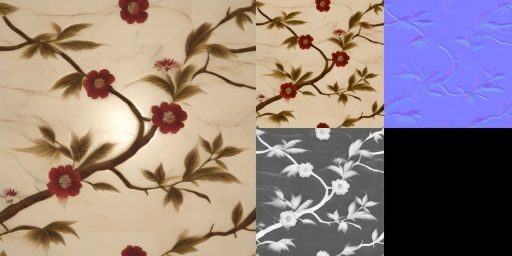} &
  \includegraphics[width=\SupWidthTxt]{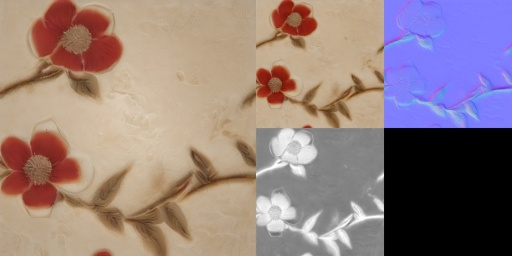} &
  \includegraphics[width=\SupWidthTxt]{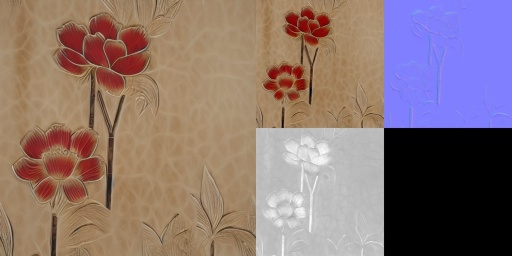} \\

  &
  \begin{minipage}{\SupWidthTxt}
    \centering
    \scriptsize\textit{a PBR material of ground, artistic} 
  \end{minipage} &
  \begin{minipage}{\SupWidthTxt}
    \centering
    \scriptsize\textit{a PBR material of fabric} 
  \end{minipage} &
  \begin{minipage}{\SupWidthTxt}
    \centering
    \scriptsize\textit{a PBR material of tile, marble} 
  \end{minipage} &
  \begin{minipage}{\SupWidthTxt}
    \centering
    \scriptsize\textit{a PBR material of wall, cement} 
  \end{minipage} &
  \begin{minipage}{\SupWidthTxt}
    \centering
    \scriptsize\textit{a PBR material of leather} 
  \end{minipage} \\
  \noalign{\smallskip}

  \includegraphics[width=1.6cm]{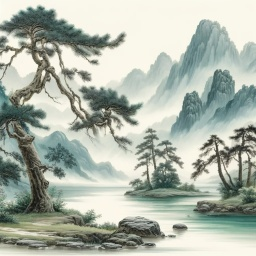} &
  \includegraphics[width=\SupWidthTxt]{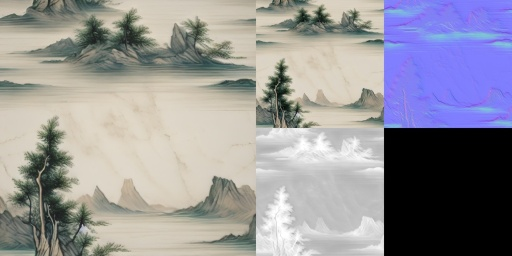} &
  \includegraphics[width=\SupWidthTxt]{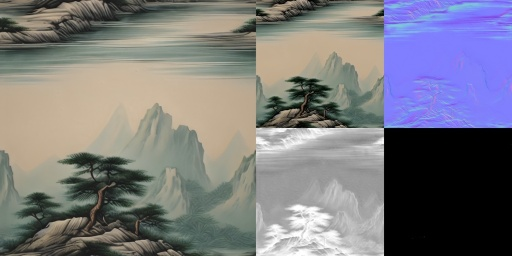} &
  \includegraphics[width=\SupWidthTxt]{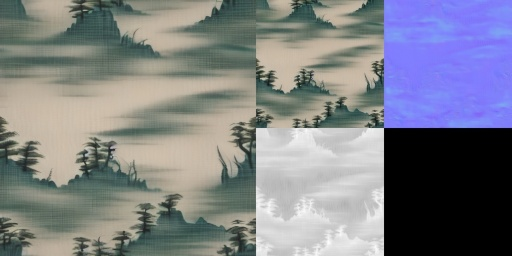} &
  \includegraphics[width=\SupWidthTxt]{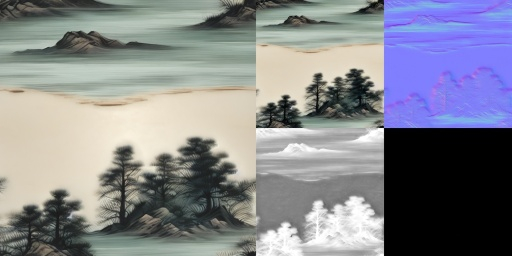} &
  \includegraphics[width=\SupWidthTxt]{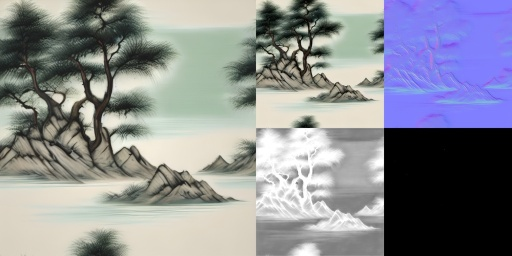} \\

  &
  \begin{minipage}{\SupWidthTxt}
    \centering
    \scriptsize\textit{a PBR material of tile, marble} 
  \end{minipage} &
  \begin{minipage}{\SupWidthTxt}
    \centering
    \scriptsize\textit{a PBR material of wall, painted} 
  \end{minipage} &
  \begin{minipage}{\SupWidthTxt}
    \centering
    \scriptsize\textit{a PBR material of fabric} 
  \end{minipage} &
  \begin{minipage}{\SupWidthTxt}
    \centering
    \scriptsize\textit{a PBR material of tile, painted, artistic} 
  \end{minipage} &
  \begin{minipage}{\SupWidthTxt}
    \centering
    \scriptsize\textit{a PBR material of ground, polished} 
  \end{minipage} \\

\end{tabular}
\egroup
\caption{Additional results for style control.}
\Description{}
\label{fig:style_supple}
\end{figure*}

% style control
\begin{figure*}[tb]
  \centering
  \bgroup
  \includegraphics[width=0.82\linewidth]{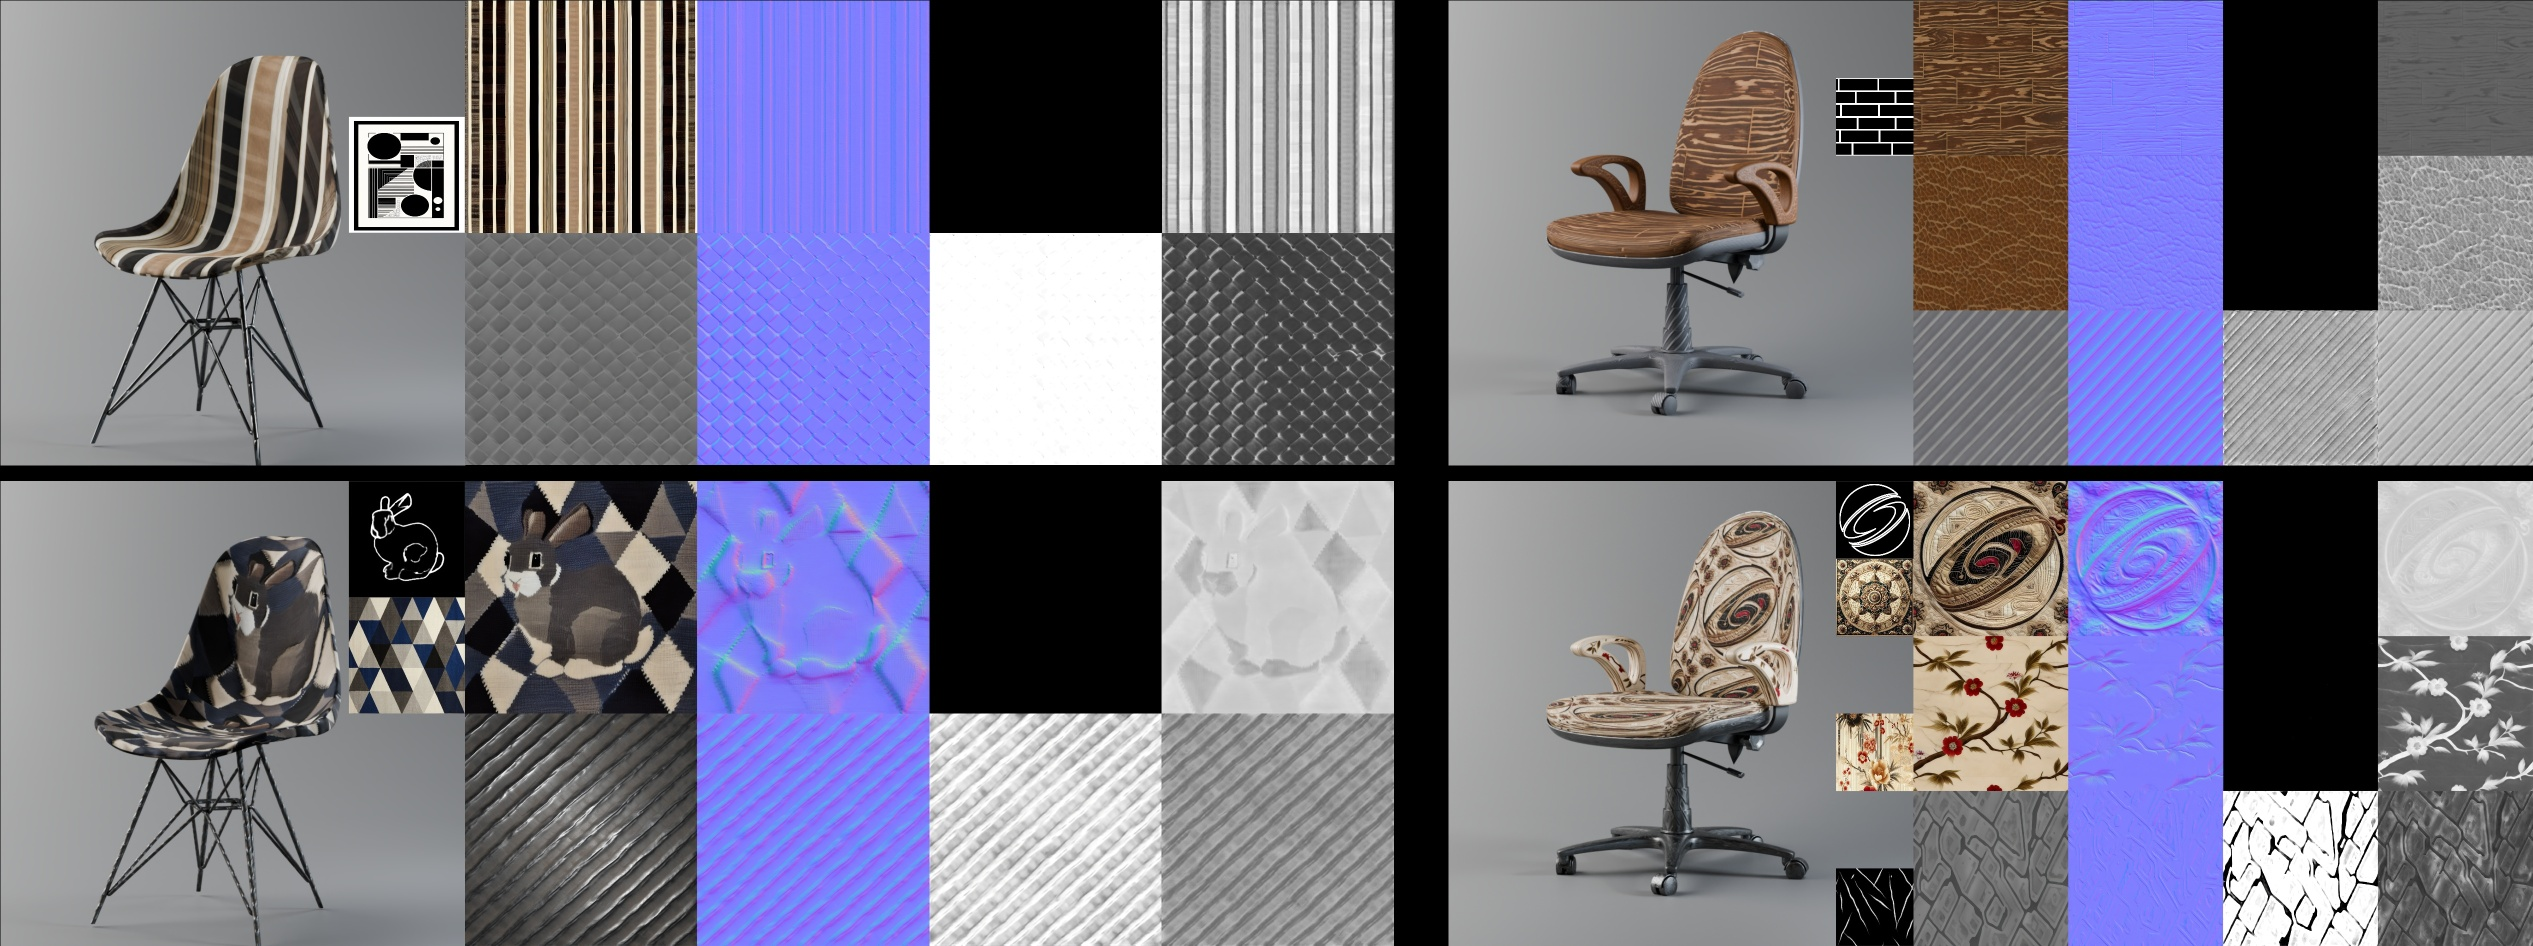} \\
\egroup
\caption{Additional results for shape control.}
\Description{}
\label{fig:shape_supple}
\end{figure*}
